# Supplementary material for: TraveL: Transformer-based Multi-view Path Distributional Representation Learning
Source: arXiv:2609.03427 source file (2026-09-03)
Supplement: Supplementary file 1 [file appendix.tex]

\clearpage
\section{Kolmogorov–Smirnov Test}
Kolmogorov–Smirnov Test is a classic nonparametric test of the equality of two continuous one-dimensional probability distributions based on two sets of values sampled from the two distributions respectively. 
More specifically, K-S test transforms each set of sampled values to an empirical distribution function, i.e., $F_n(x)$ for the generated travel time set $S^\prime_p$ in this work, and $F_m(x)$ for the historical travel time set $S_p$, respectively. Formally, we have,
\begin{equation}
F_n(x) = \frac{1}{n}\sum^n_{i=1}{\textbf{1}_{[-\infty, x]}(X_i)}
\end{equation}
where $X_i$ is the $i$-th smallest value in $S^\prime_p$, $\textbf{1}_{[-\infty, x]}(X_i)$ is the indicator function, equal to 1 if $X_i \leq x$ and equal to 0 otherwise. And similarly, we obtain $F_m(x)$ from $S_p$.
Then K-S test defines the K-S distance between two sample sets,  as follows, 
\begin{equation}
KS(S^\prime_p, S_p) = {\sup}_x|F_n(x)-F_m(x)|
\end{equation}
which is then exploited to judge whether the two sample sets are from a same distribution.





\section{Real-world Dataset Preprocesssing}
For Porto and Tokyo, we obtain the on-path sequences from the trajectories via Barefoot, a Hidden
Markov Model–based model~\cite{newson2009hidden}, to relocate each GPS sample point in the trajectory on a road segment and estimate the travel time spent on each road segment under the assumption that the moving speed between two consecutive sample points is constant. As such, a trajectory dataset is transformed into an on-path sequence dataset.

Furthermore, we exploit the three-sigma principle to remove outlier on-path sequences, i.e., on-path sequences which contain a road segment with outlier travel time are removed. Here we fit the travel time distribution on each road segment to a log-normal distribution~\cite{li2013empirical}, and we regard the travel time away from the average travel speed for more than three standard deviation as outliers. 




\section{Synthetic Dataset Generation}
To deal with the data sparsity issue, we propose to build a synthetic dataset, Syn-Porto, where each path can be covered by a larger number of on-path sequences.
The generation of Syn-Porto has three steps: i) generate the origin-destination (OD) pairs on Porto, ii) generate paths between OD pairs and iii) generate travel times on the paths. Inspired by Simfleet~\footnote{Simfleet can be found at https://github.com/javipalanca/simfleet.}, we build a simulation system with \textit{N} drivers randomly initialized at the map in Porto and a passenger generated at the map every \textit{T} time slots, following an \textit{Origin Sampling Strategy}. Each passenger sends requests to all free drivers (if there is no free driver, the passenger waits for the first free driver) and the nearest (e.g., with the shortest distance along a sequence of consecutive road segments) free driver drives to the passenger and serves him. 
After the driver takes the passenger, the passenger tells the driver a destination following a \textit{Destination Sampling Strategy} and then the drivers drives to the destination. 
Here the Origin Sampling Strategy is used to generate possible locations of a passenger and the Destination Sampling Strategy is used to generate possible destinations. A naive design of the Origin or Destination Sampling Strategy is to randomly select a road segment in the road segment with equal probability. However, this naive design may be too far from the real-world scenarios. Another idea is to generate the origins and destinations by sampling road segments based on the distribution of their occurrences in the real-world datasets. However, not all the road segments are covered in the real-world trajectories, so that those road segments may be never seen in the synthetic dataset (which is not our goal).
Thus, we propose to explore the information in the real-world datasets to benefit the generation of origins and destinations, with an exploration rate $r$ applied.
More specifically, every time we want to sample an origin or a destination, we have the probability of $(1-r)$ to sample from the origin/destination distribution in the real-world Porto dataset, and the probability of $r$ to randomly sample an origin or a destination from all road segments.
To distinguish the number of passengers in rush hours (i.e., 8-10AM and 5-7PM) and normal hours, we set a smaller \textit{T} in rush hours (denoted as \textit{$T_{Rush}$}) than that in normal hours (denoted as \textit{$T_{Norm}$}). 

After an OD pair is generated, we generate the top-k shortest paths, top-k fastest paths and top-k fuel-efficient paths (traffic speed here is estimated as the speed limit and the fuel cost is estimated via~\cite{guo2012ecomark, guo2015ecomark}, similar to PathRank~\cite{yang2019pathrank}) and randomly select one as the path the driver drives along. 
Finally, we generate the travel time spent on each road segment along the top-k shortest paths. We exploit the speed limit as a base to generate the synthetic travel speed distribution: i) the travel speed distribution is assumed to be a normal distribution or a log-normal distribution~\cite{rakha2006estimating}; ii) the $\mu_{Rush}$ in normal hours and the $\mu_{Norm}$ in rush hours are set to be the speed limit; and iii) $\sigma_{Rush}$\% of the speed limit used as the 3$\sigma$ for either log-normal or normal distribution in rush hour, while $\sigma_{Norm}$\% of the speed limit is used as $3\sigma$ for normal hour.




As the default setting, we have the number of drivers in the road is 100, $T_{Norm}$ = 1 minute, $T_{Rush}$ = 10 seconds, $r$=0.1, $k$=10, $\sigma_{Rush}$=5 and $\sigma_{Norm}$=15 in our experiments. 
The setting of these parameters is based on the analysis of the Porto trajectory dataset and the conclusion of some literature, claiming that the travel speed distribution on a road segment may be well fit to a normal or log-normal distribution. 
To explore the impact of the assumption of travel speed distribution to the experimental results, we create three versions of Syn-Porto, denoted as $D_{nor}$, $D_{logn}$ and $D_{mix}$ respectively, with road segment travel times sampled from a Normal distribution, a Log-normal distribution, or a mixture of them.
Each version contains 1 million paths, each of which has one hundred on-path sequences departing at normal hours and one hundred sequences departing at rush hours.
We evaluate TraveL on all the three versions to validates its effectiveness under various assumptions.


\begin{figure}[t]
\centering
\includegraphics[width=3.3in]{Figures/hyper-sens-ttde.PNG}
\hup\hup
\caption{Parameter Sensitivity Test for TTDE} 
\label{fig:hyper-sens-ttde}
\end{figure}

\section{Optimal Parameter Settings}
For TraveL, we have the following optimal parameter setting: i) the number of multi-view regional attention layers (denoted as $L$ in Appendix) in Multi-view Path Transformer as 6; ii) the number of hops in Hop-view (denoted as $H$) as 3; iii) the dimensionality of both $\mu_p$ and $\sigma_p$ (denoted as $D$) as 128; and vi) the number of sample points (denoted as $N$) from the distributional representation as 100. 
For Syn-porto, we have $\lambda_1$ as 0.3, $\lambda_2$ as 0.0 (since synthetic data does not face the data sparsity issue), $\lambda_3$ as 0.7, $\lambda_4$ as 0.1 and $\lambda_5$ as 0.05 to weight the loss. For the two real-world datasets, we have $\lambda_1$ as 0.1, $\lambda_2$ as 0.3, $\lambda_3$ as 0.6, $\lambda_4$ as 0.1 and $\lambda_5$ as 0.05. We also conduct a parameter sensitivity test to evaluate the impacts of these parameters to the model performance, which is shown in the following section.




\section{Parameter Sensitivity Test}
In this section, we conduct a sensitivity test of the parameters to evaluate their impacts on the TraveL performance. 
We test the parameter sensitivity of TraveL on $D_{mix}$, Porto and Tokyo for all the three tasks, i.e., travel time distribution estimation, path similarity prediction and destination prediction. 
While our optimal parameters are selected by minimizing the losses instead of observing the performance on specific tasks for tuning, we still would like to evaluate how the parameter setting influences the model performance.
To test the parameter sensitivity of TraveL, we vary the values of the parameters, 1) the number of multi-view regional attention layers, i.e., $L$, as 2, 4, 6 and 8; 2) the number of hops in Hop-view, i.e., $H$, as 2, 3, 4 and 5; 3) the dimensionality of TraveL distributional representation, i.e., $D$, as 64, 128, 256 and 512; 4) the number of sample points, i.e., $N$, from the distributional representation as 50, 75, 100, 125. 
We show the results in Figure~\ref{fig:hyper-sens-ttde}, Figure~\ref{fig:hyper-sens-psp} and Figure~\ref{fig:hyper-sens-dp} for the TTDE, the PSP and the DP task, respectively.

As shown, the optimal parameter settings, i.e., $\{L=6, H=3, D=128, N=100\}$ overall achieve great performances on all the three tasks. Meanwhile, we observe that there are some special cases, such as for TTDE and $D_{mix}$, setting $D=256$ without changing other parameters reduce the MKS from 0.29 to 0.27 (which is the MKS when $D=128$). Besides, an interesting observation is, by increasing $L$ from 6 to 8 always leads to a worse performance on all three tasks for the real-world datasets, i.e., Porto and Tokyo. By contrast, on $D_{mix}$, the performance of TraveL is improved when $L$ increases from 6 to 8. The reason may be that, the amount of data in the synthetic dataset is larger, than that in the real-world datasets, and the larger amount of data can support the training of a deeper neural network structure. Though, we observe that the optimal parameter setting still performs well on $D_{mix}$, i.e., achieving either the best or the second best result.


\vspace{0.1in}
\begin{figure}[b]
\centering
\includegraphics[width=3.3in]{Figures/hyper-sens-psp.PNG}
\hup\hup
\caption{Parameter Sensitivity Test for PSP} 
\label{fig:hyper-sens-psp}
\end{figure}



\begin{figure}[b]
\centering
\includegraphics[width=3.3in]{Figures/hyper-sens-dp.PNG}
\hup\hup
\caption{Parameter Sensitivity Test for DP} 
\label{fig:hyper-sens-dp}
\end{figure}
